# Supplementary material for: Locating the missing superconducting electrons in overdoped cuprates
Source: arXiv:1802.02101 source file (2019-05-04)
Supplement: Supplementary file 1 [file SI.pdf]

# Supplementary Material: Locating the missing superconducting electrons in the overdoped cuprates $La_{2-x}Sr_xCuO_4$

Fahad Mahmood,[1] Xi He,[2,3] Ivan Božović,[2,3] and N. P. Armitage[1]

[1] *The Institute for Quantum Matter, Department of Physics and Astronomy, The Johns Hopkins University, Baltimore, MD 21218 USA.*
[2] *Brookhaven National Laboratory, Upton, NY 11973, USA.*
[3] *Applied Physics Department, Yale University, New Haven, Connecticut 06520, USA.*

## A. Methods

The complex conductivity was determined by time-domain THz spectroscopy. A femtosecond laser pulse is split along two paths and excites a pair of photoconductive 'Auston'-switch antennae grown on LT-GaAs wafers. A broadband THz range pulse is emitted by one antenna, transmitted through the LSCO film, and measured at the other antenna. By varying the length-difference of the two paths, we map out the entire electric field of the transmitted pulse as a function of time. Comparing the Fourier transform of the transmission through LSCO to that of a reference resolves the full complex transmission. We then invert the transmission to obtain the complex conductivity via the standard formula for thin films on a substrate:

$$\tilde{T}(\nu) = \frac{1+n}{1+n+Z_0\tilde{\sigma}(\nu)d}e^{i\Phi_s} \quad (1)$$

where $\Phi_s$ is the phase accumulated from the small difference in thickness between the sample and reference substrates and $n$ is the substrate index of refraction. $n$ is determined by an independent measure of the complex transmission of the reference substrate while $\Phi_s$ is determined by setting $\sigma_2(\nu) = 0$ in the complex transmission at room temperature ($T = 295\,\text{K}$), which is the case for frequencies much less than the scattering rate. By measuring both the magnitude and phase of the transmission, this inversion to conductivity is done directly and does not require a Kramers-Kronig transformation.

The LSCO films were deposited on 1-mm-thick single-crystal $LaSrAlO_4$ substrates, epitaxially polished perpendicular to the (001) direction, by atomic-layer-by-layer molecular-beam-epitaxy (ALL-MBE). The samples were characterized by reflection high-energy electron diffraction, atomic force microscopy, X-ray diffraction, and resistivity and magnetization measurements, all of which indicate excellent film quality. All the films studied in this work are 20 monolayers thick (one monolayer is $\approx 6.6\,\text{Å}$).

The superfluid spectral weight in the delta function $S_\delta$ is determined by a two-coil mutual inductance technique. For a superconducting film of thickness $d$ and infinite radius placed between two coils of radii $R_1$ and $R_2$ parallel to one another and separated by a distance $D$, the complex mutual inductance can be written as:

$$\begin{aligned}\hat{M} &= \text{Re}M + i\text{Im}M \\ &= \mu_0\pi R_1R_2\frac{\int_0^\infty d\mathbf{q}[\exp(-\mathbf{q}D)J_1(\mathbf{q}R_1)J_1(\mathbf{q}R_2)]}{\cosh(Qd) + [(Q^2+\mathbf{q}^2)/2\mathbf{q}Q]\sinh(Qd)}\end{aligned}$$

where $\mathbf{q}$ is the wave-vector, $J_1(x)$ is the first order Bessel function, $Q^2 = q^2 + (1/\lambda^2) - i\mu_0\omega\sigma_1$ and $\sigma_2 = 1/\mu_0\omega\lambda^2$. This can be generalized to the case of two solenoids with $N_1$ and $N_2$ turns respectively by the summation over each pair of coils. Re$M$ and Im$M$ are measured experimentally and the above equation is numerically inverted using the algorithm outlined by He, X., et. al. (Review of Scientific Instruments 87, 113903 2016). to obtain $\lambda$ and $\sigma_1$ from which the superfluid spectral weight is calculated as $S_\delta = \frac{1}{2\pi\mu_0\lambda^2}$. Further details on the mutual inductance setup can be obtained in the Methods section of Ref. 13.

## B. Measured complex conductivity for all films

Here we present the measured raw data, $\sigma_1(\nu)$ and $\sigma_2(\nu)$, for each film studied in this work at various temperatures (Fig. S1). The results for the film with the $T_c = 27.5\,\text{K}$ are shown in Fig. 1a,b of the main text. $\sigma_1(\nu)$ and $\sigma_2(\nu)$ are extracted from the measured complex transmission $\tilde{T}(\omega)$ as outlined in the Methods section above.

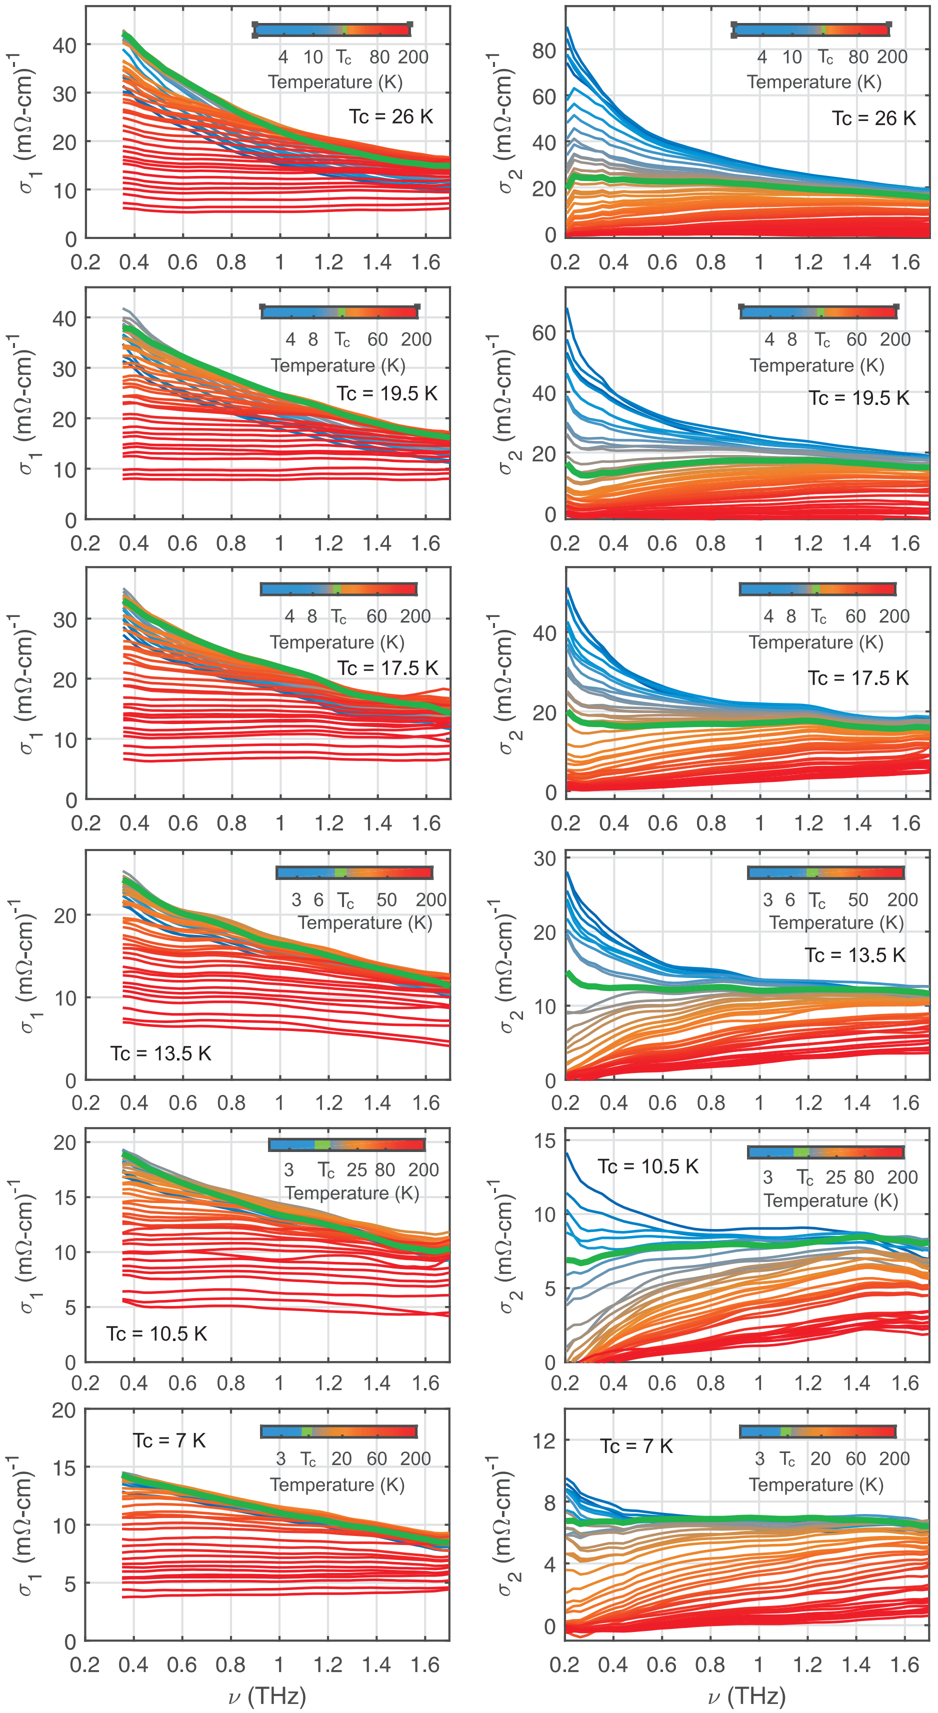


FIG. S1: THz optical conductivity of various overdoped $La_{2-x}Sr_xCuO_4$ thin films at different temperatures. The $T_c$ of each film is indicated within each panel

### C. Fits to extract $S_u$ and $S_n$ from $\sigma_1(\nu)$

As discussed in the main text, $\sigma_1(\nu)$ for each film can be fit to a single Drude to extract the uncondensed ($S_u$) and normal state ($S_n$) spectral weight along with the scattering rate ($\tau$). The fits for films with $T_c = 27.5\,\mathrm{K}$, 13.5 K and 7 K are shown in Fig. 2a, 2b and 2c of the main text, respectively. The fits for the other four films are shown here in Fig. S2.

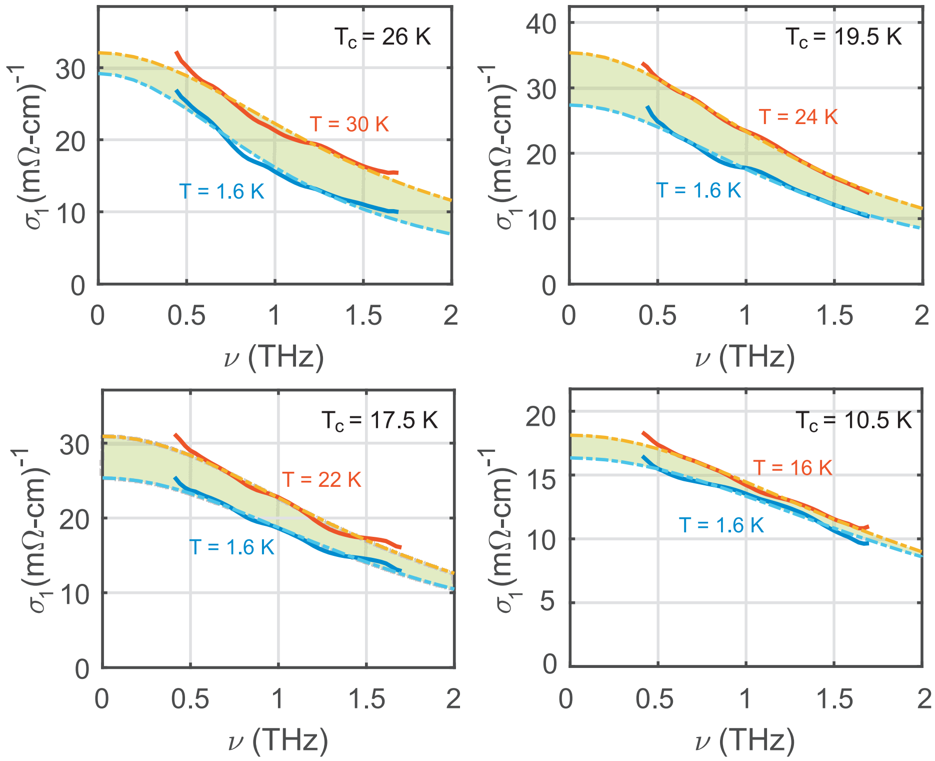


FIG. S2: Fits to extract $S_u$ and $S_n$ from $\sigma_1(\nu)$. Comparison of the real part of the optical conductivity above and below $T_c$ for three of the $La_{2-x}Sr_xCuO_4$ films. Data for the other three films are presented in the main text. Solid lines indicate the TDTS data. Dashed lines show a Drude fit with a single scattering rate i.e. $\sigma_1(\nu) = S\tau/(1+\nu^2\tau^2)$. Shaded green region represents the expected superfluid spectral weight.

### D. Contribution to $\sigma_2(\nu)$ from high frequency absorption

In this section we study whether absorption at frequencies much greater than the setup's spectral range contributes to the measured imaginary part of the complex conductivity i.e. $\sigma_{2,m}(\nu)$. Such excitations will give a contribution to the low frequency dielectric constant that should be removed from $\sigma_{2,m}(\nu)$ before converting it to a phase stiffness. Due to the Kramers-Kronig relation for optical conductivity as stated below, a finite $\sigma_{1,m}(\nu)$ at high frequencies (absorption) can lead to a measurable $\sigma_{2,m}(\nu)$ at low frequencies:

$$\sigma_{2,m}(\nu) = -\frac{2\nu}{\pi}\mathcal{P}\int_0^\infty \frac{\sigma_{1,m}(\nu')}{\nu'^2-\nu^2}\mathrm{d}\nu' \tag{2}$$

To consider if that is the case in our measurements, we study the metallic normal state conductivity of the films $\sim 50\,\mathrm{K}$ above $T_c$. As noted in the main text, the normal state $\sigma_{1,m}(\nu)$ at low frequencies is Drude-like and so the low frequency complex conductivity can be written as:

$$\sigma(\nu) = \frac{S\tau}{1-i\nu\tau} + iE(\nu) = \sigma_{1,d}(\nu) + i\sigma_{2,d}(\nu) + iE(\nu) \tag{3}$$

where $\sigma_{1,d}(\nu) = S\tau/(1+\nu^2\tau^2)$, $\sigma_{2,d}(\nu) = S\nu\tau^2/(1+\nu^2\tau^2)$, and $E(\nu)$ is a real negative function. In Fig. S3, we plot $\sigma_{1,m}(\nu)$ and $\sigma_{2,m}(\nu)$ for each film measured at $\sim 50\,\mathrm{K}$ above $T_c$. $\sigma_{1,m}(\nu)$ for each film can be fit to $\sigma_{1,d}(\nu)$

to extract the parameters $S$ and $\tau$ from which $\sigma_{2,d}(\nu)$ is calculated. As can be seen, the measured imaginary conductivity $\sigma_{2,m}(\nu)$ does not match the calculated imaginary conductivity $\sigma_{2,d}(\nu)$, i.e., $\sigma_{2,m}(\nu) \neq \sigma_{2,d}(\nu)$, for films with $T_c = 27.5\,\mathrm{K}$ and $T_c = 26\,\mathrm{K}$ indicating that $E(\nu) \neq 0$ for these films. We find that for the metallic normal state $E(\nu) = \sigma_{2,m}(\nu) - \sigma_{2,d}(\nu)$ is independent of temperature within experimental uncertainty. Based on this, we make the reasonable assumption that the contribution of high-frequency absorption to $\sigma_{2,m}(\nu)$ below $T_c$ is given by the function $E(\nu)$ as determined at $\sim 50\,\mathrm{K}$ above $T_c$ e.g. the temperature dependent changes to $E(\nu)$ are small. Based on this, $\nu\sigma_2$ plotted in Fig. 4a for $T = 1.6\,\mathrm{K}$ in the main text is determined using $\sigma_2 = \sigma_{2,m} - E(\nu)$ to subtract out the high-frequency absorption contribution. Note that for films with $T_c = 19.5\,\mathrm{K}, 17.5\,\mathrm{K}$, $13.5\,\mathrm{K}$, $10.5\,\mathrm{K}$, and $7\,\mathrm{K}$, $E(\nu) \approx 0$. Unnormalized $\nu\sigma_2$ (corrected with the $E(\nu)$ function) is plotted in Fig. S4.

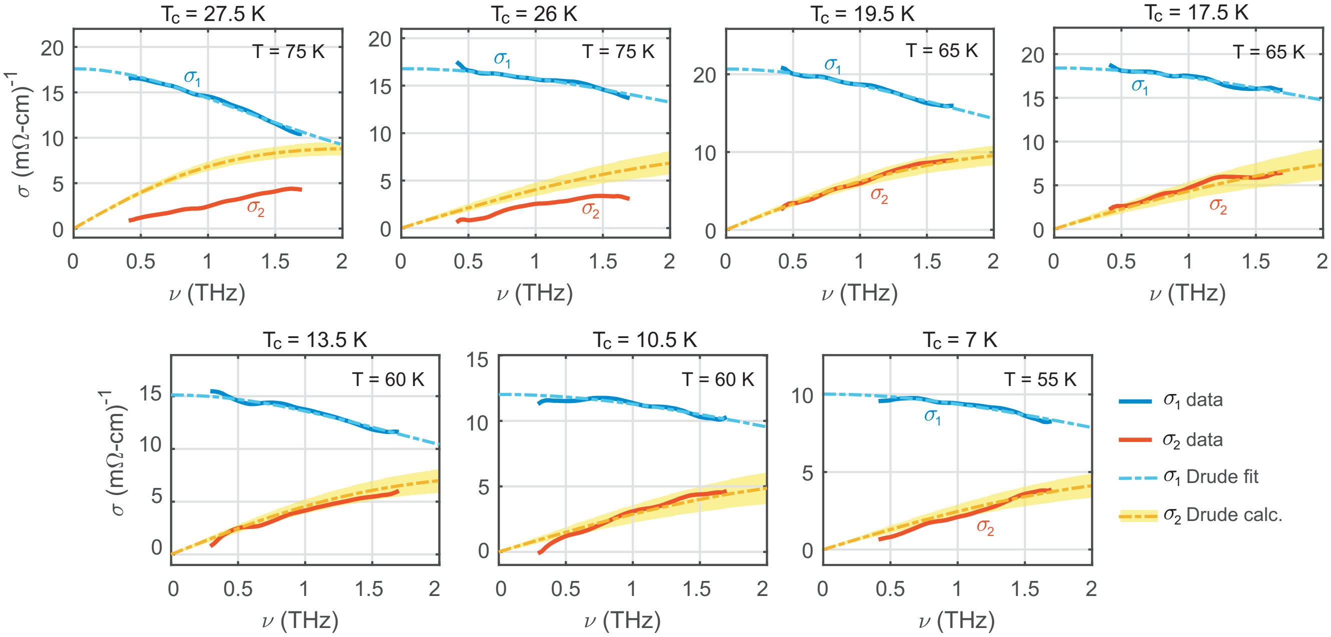


FIG. S3: Determining $E(\nu)$, the contribution to $\sigma_2(\nu)$ from high frequency absorption. For each film the measured $\sigma_{1,m}(\nu)$ at $\sim 50\,\mathrm{K}$ above $T_c$ is fit to a single Drude peak $S\tau/(1+\nu^2\tau^2)$ (blue dashed line). The resulting $\sigma_{2,d}(\nu) = S\nu\tau^2/(1+\nu^2\tau^2)$ is calculated and plotted as the orange dashed line with the shaded yellow region representing the 95% confidence interval in determining $\sigma_{2,d}(\nu)$ from the fitting parameters. $E(\nu)$ is given by $\sigma_{2,m}(\nu) - \sigma_{2,d}(\nu)$ for the films with $T_c = 27.5\,\mathrm{K}$ and $T_c = 26\,\mathrm{K}$.

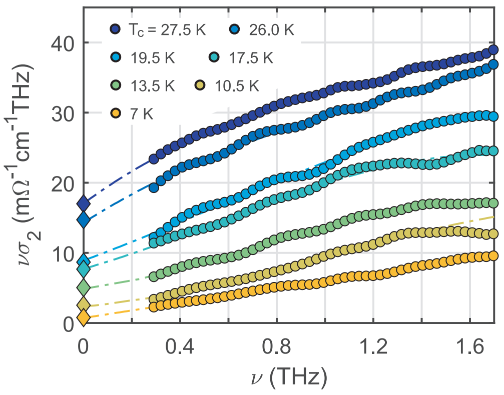


FIG. S4: $\nu\sigma_2$ versus frequency for all films at $T = 1.6\,\mathrm{K}$. $\nu\sigma_2$ is proportional to the superfluid phase stiffness $\mathcal{T}_\phi$. Circle and diamond symbols represent the TDTS and two-coil mutual inductance data respectively. Dashed lines are guides to the eye.

### E. Kramers-Kronig compatible analysis of $\sigma_1(\nu)$ and $\sigma_2(\nu)$

In our TDTS experiments, $\sigma_1(\nu)$ and $\sigma_2(\nu)$ are measured independently of each other. $\sigma_1(\nu)$ is then fit to a single Drude to extract the spectral weight and the scattering rate. To increase confidence in these fits, we show here that the measured $\sigma_2(\nu)$ is indeed compatible with the calculated $\sigma_2(\nu)$ from the Kramer-Kronig transform of the fitted $\sigma_1(\nu)$.

Figure S5 shows this comparison for the normal state data. For each film, the measured normal state $\sigma_1(\nu)$ is fit to a single Drude, i.e., $S\tau/(1+\nu^2\tau^2)$ to obtain $S$ and $\tau$ (also shown in Fig. 2 and Fig. S2). The resulting $\sigma_2(\nu)$ is then calculated as $S\nu\tau^2/(1+\nu^2\tau^2)$ (Kramers-Kronig transform of the fitted $\sigma_1(\nu)$) and plotted as the orange dashed line to compare with the measured $\sigma_2(\nu)$ (red line). Note that the measured $\sigma_2(\nu)$ for the films with $T_c = 27.5\,\mathrm{K}$ and $T_c = 26\,\mathrm{K}$ is adjusted with the $E(\nu)$ function as discussed above in section C. As shown in Fig. S5, there is excellent agreement between the measured and calculated $\sigma_2(\nu)$.

For the superconducting state, the measured quantity of interest is $\nu\sigma_2$ as shown in Fig. 4a and Fig. S4. To see if this is consistent with the fitting to the residual $\sigma_1(\nu)$, we calculate $\nu\sigma_2$ as follows:

$$\nu\sigma_2 = S_\delta + \frac{S_u\nu^2\tau^2}{1+\nu^2\tau^2} \tag{4}$$

where $S_\delta$ is the spectral weight in the superconducting state from MI measurements and the second term corresponds to the Kramers-Kronig transform of the fit to the measured $\sigma_1(\nu)$ at 1.6 K as shown in Fig. 2 and Fig. S2. We compare this calculated $\nu\sigma_2$ with the measured $\nu\sigma_2$ in Fig. S6. There is reasonably good agreement between the two for each film. Differences are likely due to small deviations from the exact Drude form for $\sigma_1(\nu)$. The systematic error for the film with $T_c = 27.5\,\mathrm{K}$ is likely due to the error in the estimation of the $E(\nu)$ function.

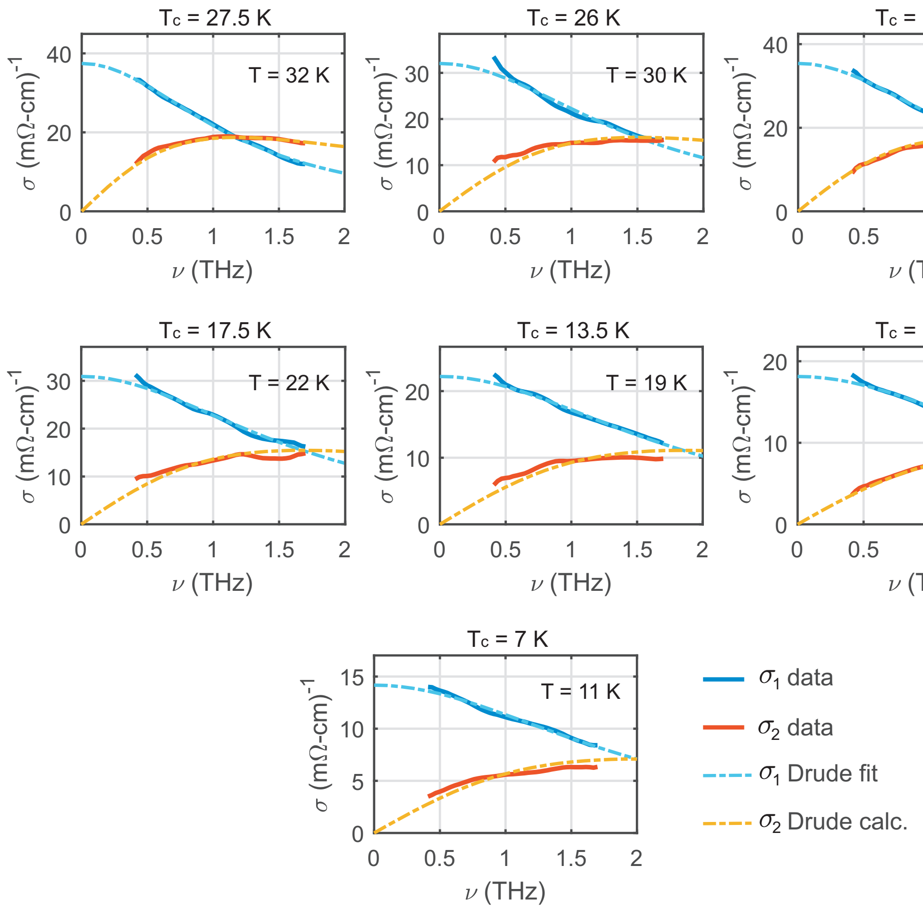


FIG. S5: Comparison of the measured and calculated normal state $\sigma_2$ for each film

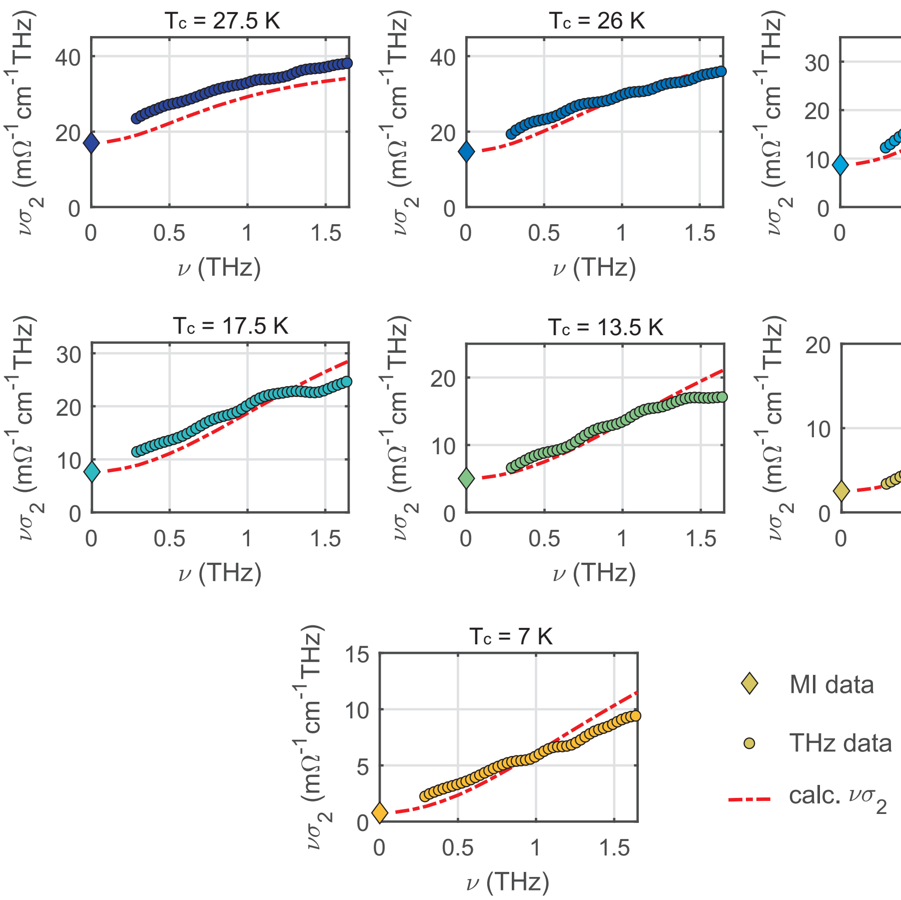


FIG. S6: Comparison of the measured and calculated $\nu\sigma_2$ at $T = 1.6\,\mathrm{K}$ for each film

## F. Spectral weights in absolute units

Figure 2e of the main text shows the residual ($S_u$) and superfluid ($S_\delta$) spectral weights, normalized to the normal state ($S_n$) spectral weight, as a function of $T_c$. Here we plot the absolute spectral weights $S_n$, $S_u$ and $S_\delta$ for each film (Fig. S7). In addition, we also plot the superfluid spectral weights for the films studied by Božović et.al. [Ref. 13] as $S_{\delta,(\mathrm{ref.13})}$. This curve corresponds to the "ideal" relationship between the superfluid density and $T_c$ for overdoped $La_{2-x}Sr_xCuO_4$ films. As can be seen, all the films presented in this work lie on this "ideal" curve.

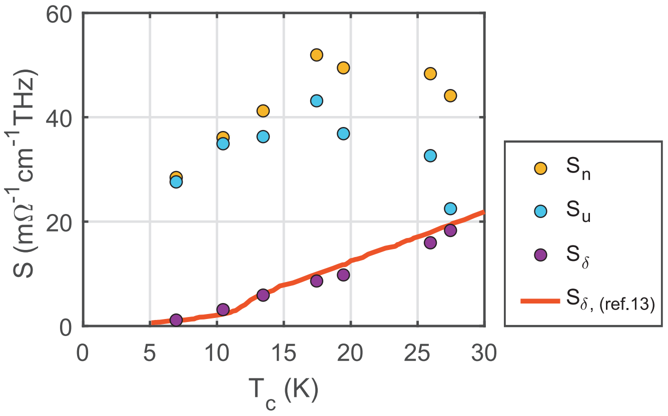


FIG. S7: Spectral weights in absolute units as a function of $T_c$. The red line is obtained from Božović et.al. [Ref. 13]

### G. Comparison of d.c. transport and TDTS results

In this section, we compare the normal state $\nu \to 0$ real conductivity, $\sigma_1(0)$, as obtained from d.c. transport on small (300 µm by 100 µm) devices and from our TDTS experiments on large (1 cm by 1 cm) films in this work (Fig. S8). The d.c. transport results are obtained from Božović et.al. [Ref. 13] at roughly 5 K above $T_c$ for each doping. The TDTS results are from extrapolating the measured normal state $\sigma_1(\nu)$ to $\nu \to 0$ using Drude fits as shown in Fig. 2 and Fig. S2.

For the d.c. transport measurements, the films were patterned lithographically into devices of Hall-bar type, with at least 4 and up to 64 contacts. To ensure low contact resistance, these films are covered with a thin (300 nm thick) gold layer in-situ. This gold layer is subsequently removed from the 'active' device surface; it remains only under the thick gold contact pads. These patterned devices have dimensions of about 300 µm by 100 µm.

As shown in Fig. S8, the two techniques give roughly the same $\sigma_1(0)$ for lower dopings (higher $T_c$) but separate at higher dopings with $\sigma_1(0)$ measured on small devices using d.c. transport being greater than our TDTS results. We note here that all the films presented in Fig. S8 lie on the "ideal" superfluid density vs. $T_c$ curve in Fig. S7. That is, the superfluid density and $T_c$ does not seem to depend on the normal state $\sigma_1(0)$.

The discrepancy between the two methods is likely explained by oxygen vacancies. Overdoped $La_{2-x}Sr_xCuO_4$ for higher Sr concentrations is prone to the formation of oxygen vacancies. These vacancies can reduce the d.c. conductivity presumably due to an increase in scattering rate without affecting $T_c$ in any significant way. Ozone annealing can be used to shift the conductivity up as it back-fills some oxygen and was carried out for the films studied in Božović et.al. [Ref. 13]. However, ozone annealing only works well with small devices in d.c. transport experiments as oxygen diffusion is mostly lateral. Therefore, the normal state d.c. conductivity of the film devices in Ref. 13 can be considered as the best case scenario and they will naturally have a higher d.c. conductivity than the un-patterned large films used for TDTS measurements.

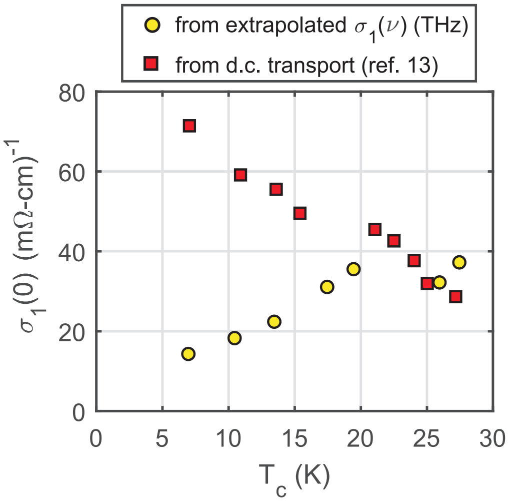


FIG. S8: Comparison of the normal state d.c. conductivity as obtained from transport experiments on small (micron) size devices and from extrapolating the measured TDTS $\sigma_1(\nu)$ for $\nu \to 0$. The d.c. transport results are obtained from Božović et.al. [Ref. 13]

### H. Superfluid spectral weight for all films

Here we present the superfluid ($S_\delta$) spectral weight for all films studied in this work as obtained from mutual inductance measurements. The results are shown in Fig. S9.

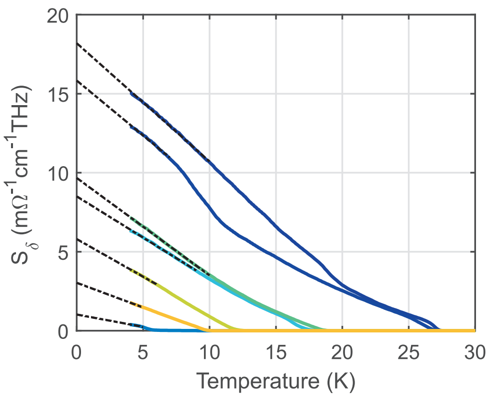


FIG. S9: The superfluid spectral weight $S_\delta$ with temperature for all films as derived from mutual inductance measurements. The dashed line represents a linear extrapolation to determine $S_\delta$ for $T = 1.6\,\mathrm{K}$.
